# Supplementary material for: sMILES SSPs: A Library of Semi-Empirical MILES Stellar Population Models with Variable [$\alpha$/Fe] Abundances
Source: arXiv:2306.05942 source file (2023-06-09)
Supplement: Supplementary file 2 [file sMILES_SSP_Paper_SupplementaryMaterials.pdf]

# Supplementary Material - Comparisons Between sMILES and Vazdekis et al. (2015) SSP and Stellar Models

Supplementary Material for the article by Knowles et al. 2023, entitled: ‘sMILES SSPs: A Library of Semi-Empirical MILES Stellar Population Models with Variable  $[\alpha/\text{Fe}]$  Abundances’.

## 1 Age and Metallicity Sequences of sMILES SSPs

Figure S1 shows a sequence of sMILES SSP spectra with ages of 2 Gyr to 14 Gyr for a fixed metallicity and a sequence of sMILES SSPs from  $[\text{M}/\text{H}]_{\text{SSP}} = -1.79$  to  $+0.26$  for a fixed age (10 Gyr), with a universal Kroupa IMF. The effect of ageing a stellar population can be mimicked by increasing the metallicity of the population at a fixed age (Worthey 1994), demonstrated by the similarity in the sequences, where old, metal-poor populations look like younger, metal-rich populations. This figure also indicates that metal poor SSPs can be distinguished from their weak absorption lines and their overall spectral shape, if well flux calibrated.

## 2 $\text{H}\beta$ and $\text{H}\beta_o$ predictions of sMILES and Vazdekis et al. (2015) SSP and Underlying Stellar Models

To supplement Section 3.2.1 (Figures 8 and 9) of Knowles et al. (2023), in Figure S2 we show the ratio of  $[\alpha/\text{Fe}]$ -enhanced and solar abundance SSP spectra in the region of  $\text{H}\beta$  and  $\text{H}\beta_o$  indices (Top panel) and over the broader region of Balmer features (Bottom panel) and highlight the Lick index definitions. There are differences between model predictions, particularly seen in spectral features found in the red pseudocontinuum bands of  $\text{H}\beta$  and  $\text{H}\beta_o$  indices. These differences lead to the differing index predictions shown in Figures 8 and 9 of Knowles et al. (2023). Spectral differences are also found for other Balmer lines but do not appear in the indices, with both models predicting an increase in index strength for increasing  $[\alpha/\text{Fe}]$  abundance ratio at all ages and metallicities tested.

To investigate causes of the different predictions from V+15 and sMILES SSP models in the  $\text{H}\beta$  region, we compare the underlying theoretical stellar models used in the SSP calculations. V+15 models are constructed using predictions of Coelho et al. (2005, 2007) stellar models and sMILES SSPs are computed from predictions of the theoretical stellar library presented in Knowles et al. (2021). It has been previously noted that different stellar models can affect predictions of  $\text{H}\beta$  and  $\text{H}\beta_o$  changes with  $[\alpha/\text{Fe}]$  (e.g. Cervantes and Vazdekis 2009; V+15), possibly due to differences in the line lists adopted for those computations. In Figure S3, we plot the ratios of an  $[\alpha/\text{Fe}]$  enhanced and a scaled-solar abundance theoretical stellar spectrum for both Coelho et al. (2005, 2007) and Knowles et al. (2021) models in the region of  $\text{H}\beta$  and  $\text{H}\beta_o$  and for a broader region of 4000-5000Å. Both sets of models were degraded and rebinned to the MILES FWHM and sampling of 2.5Å and 0.9Å, respectively. This was done for three typical stars present within a stellar population. In addition to the SSP level, differences of  $\alpha$ -enhancement predictions can also be seen at the star level for the three star types tested. These differences are then incorporated into the SSP calculations in different weights, depending on the age, metallicity and abundance pattern of the population.

## 3 $\text{Fe}5270$ , $\text{Fe}5335$ and $\text{Mg}_b$ Index Comparisons Between sMILES and Vazdekis et al. (2015) SSP Models

To supplement Section 3.2.3 of Knowles et al. (2023) in Figure S4 we compare sMILES and V+15 SSP model predictions of  $\text{Fe}5270$ ,  $\text{Fe}5335$  and  $\text{Mg}_b$  index variations with changes in  $[\text{M}/\text{H}]_{\text{SSP}}$ . For 10 Gyr old, scaled-solar (star points) and  $[\alpha/\text{Fe}]=0.4$  (triangular points) populations there is a good agreement in lower metallicity

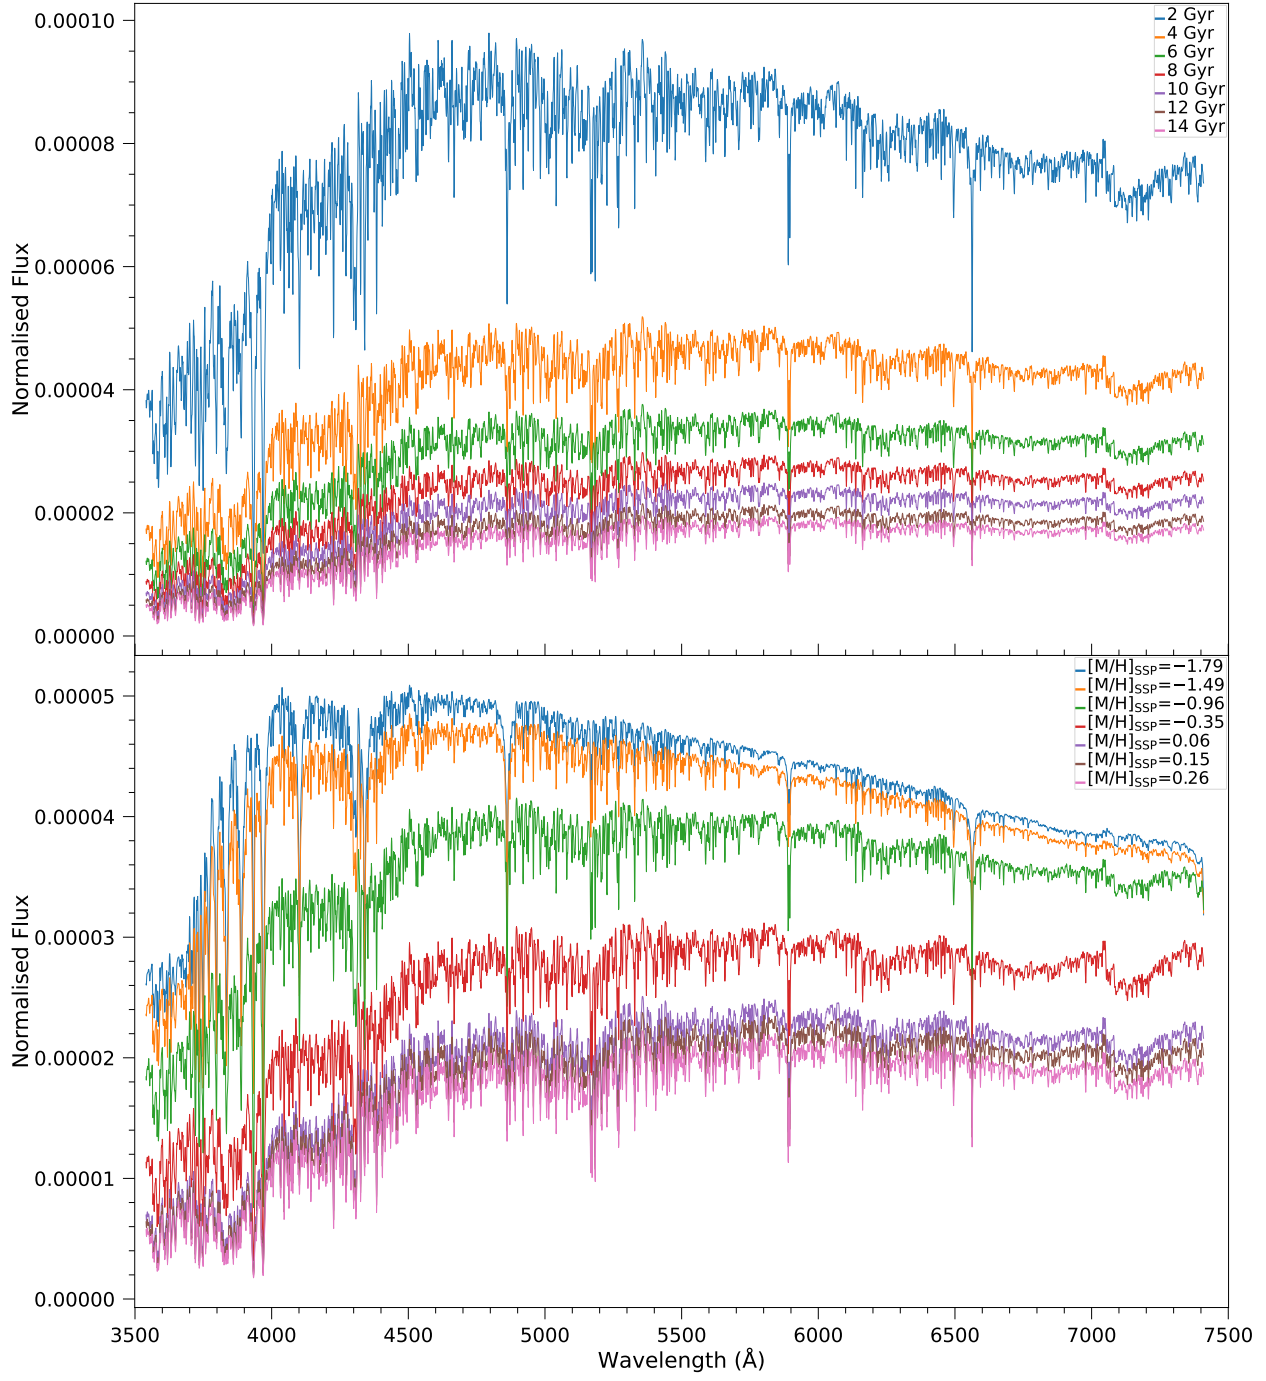

Figure S1: Top panel: sMILES SSP sequence of age for fixed metallicity ( $[M/H]_{SSP}=0.06$ ) and Universal Kroupa IMF in the full MILES wavelength range. Bottom panel: sMILES SSP sequence of metallicity for a fixed age (10 Gyr) and universal Kroupa IMF.

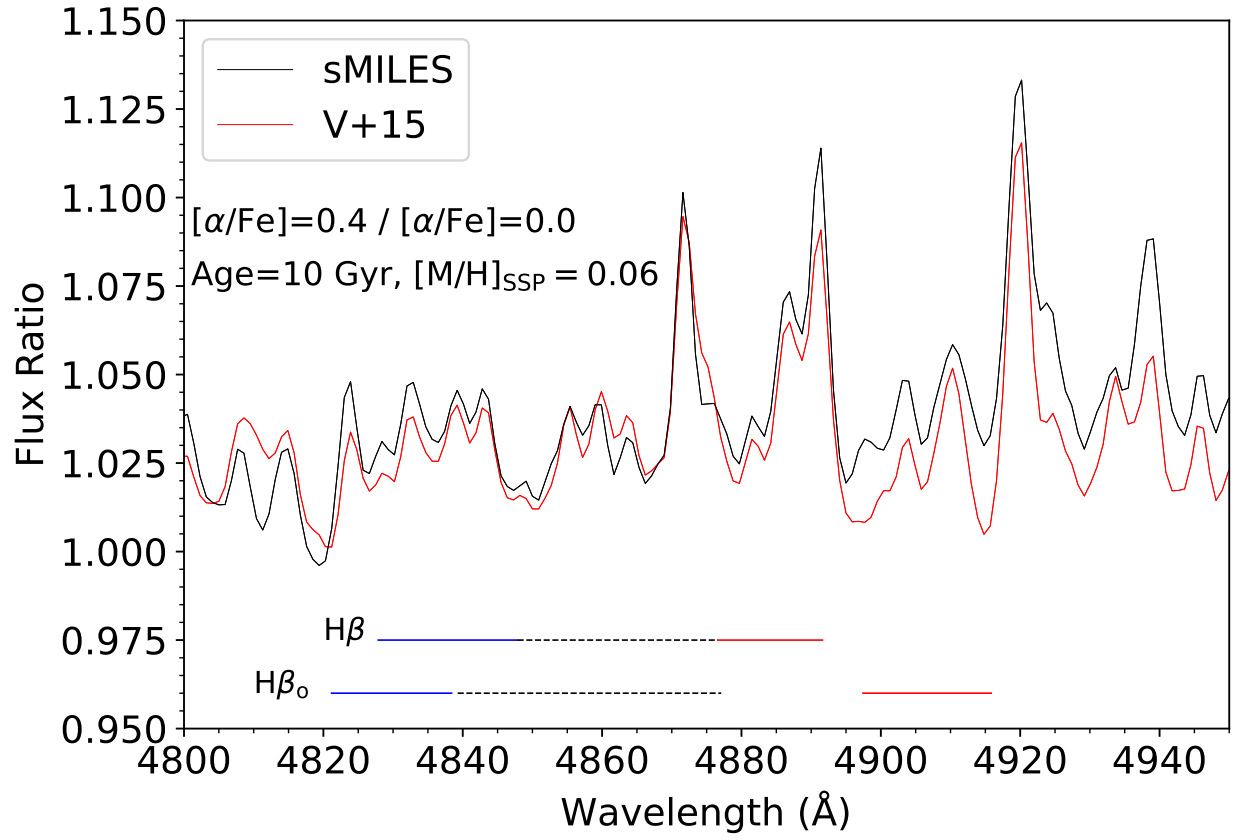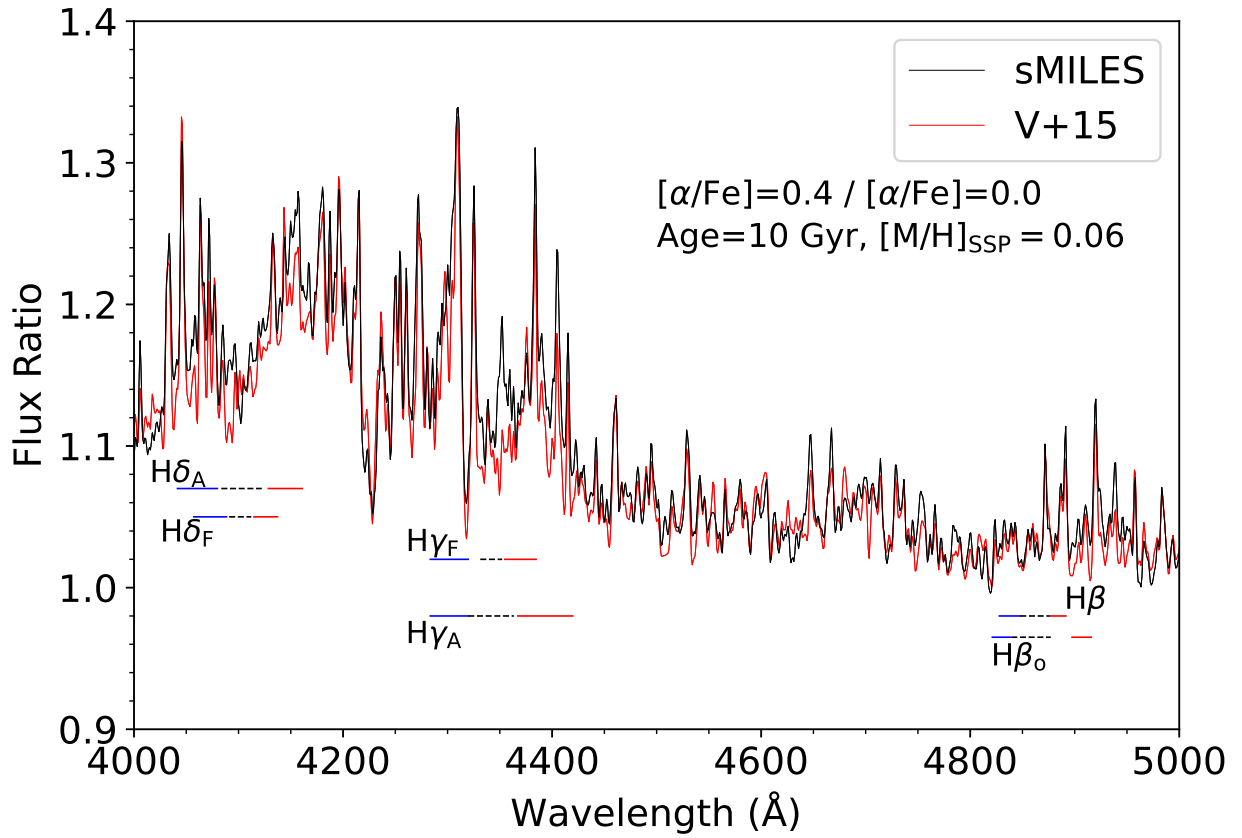

Figure S2: sMILES (black lines) and V+15 (red lines) SSP spectral predictions of changes due to  $\alpha$ -enhancements for solar metallicity and 10 Gyr populations. Top panel: For  $H\beta$  and  $H\beta_0$  index regions. Bottom panel: For 4000-5000 $\text{\AA}$ . Blue, red and feature bands of Balmer Lick index definitions are shown.

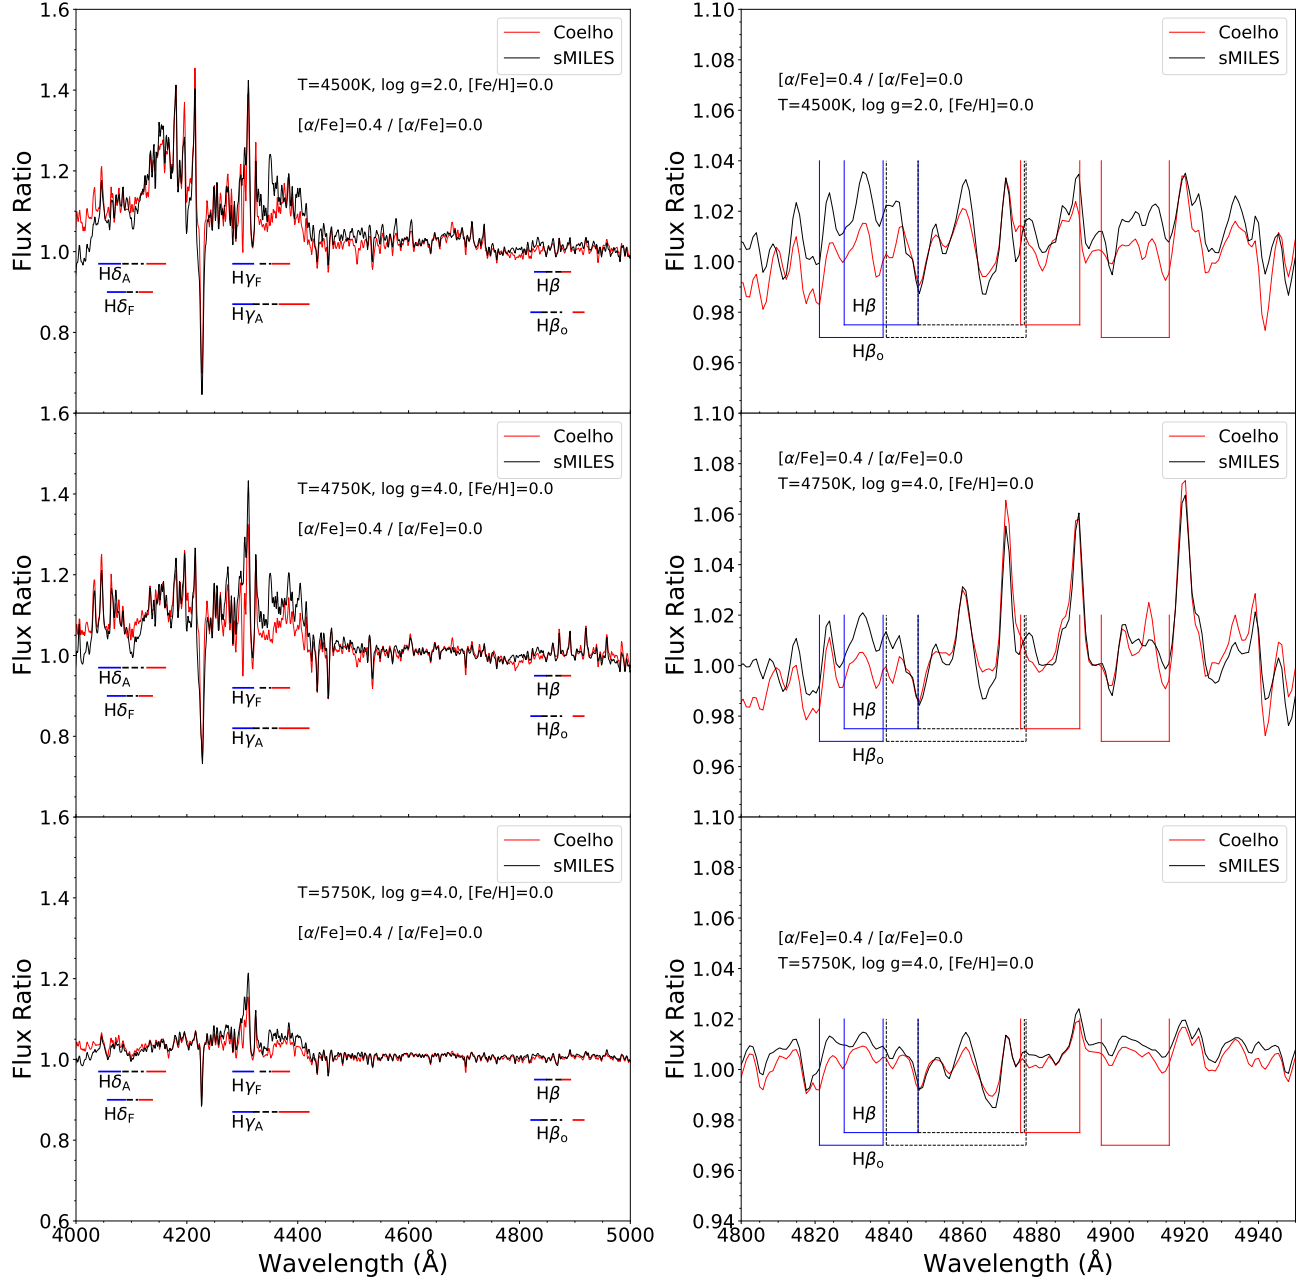

Figure S3: Predictions of changes in flux due to an  $[\alpha/\text{Fe}]$  enhancement for Coelho et al. (2005, 2007) (red lines) and sMILES (Knowles et al. 2021) (black lines) stellar spectral models, for three star types at MILES FWHM ( $2.5\text{\AA}$ ) resolution. Left panel: For 4000-5000 $\text{\AA}$ . Right panel: For  $\text{H}\beta$  and  $\text{H}\beta_0$  index regions. Blue, red and feature bands of Balmer Lick index definitions are shown.

bins and small differences in the highest metallicity bins. For the highest metallicity bins ( $[M/H]_{\text{SSP}}=0.06$  and  $[M/H]_{\text{SSP}}=0.26$ ) sMILES models predict slightly larger index strengths than the V+15 models, with differences of  $\sim 0.2\text{--}0.3$  Å.

## 4 [MgFe] and [MgFe]’ Index Comparisons Between sMILES and Vazdekis et al. (2015) SSP Models

To supplement Section 3.2.5; Table 3 and Figure 11 of Knowles et al. (2023), we compare the sMILES SSP predictions of [MgFe] and [MgFe]’ index changes with  $[\alpha/\text{Fe}]$  variations to those previously calculated with V+15 models, for  $[\alpha/\text{Fe}]=0.0$  and 0.4 populations, for the same age and metallicity ranged tested in the main article. [MgFe] and [MgFe]’ are defined in González (1993) and Thomas et al. (2003) respectively.

In Figures S5 and S6 we show the differences in [MgFe] and [MgFe]’ indices between sMILES and V+15 models for three ages and various metallicities. Calculated here are the gradients (e.g. how much the index changes with changing  $[\alpha/\text{Fe}]$ ), of the line between  $[\alpha/\text{Fe}]=0$  and 0.4 points in units of Å dex<sup>-1</sup>. As discussed in Knowles et al. (2023), both models generally agree at 7.5 and 14 Gyr old SSPs in absolute [MgFe] and [MgFe]’ strengths and in changes of values with metallicity and  $[\alpha/\text{Fe}]$  abundances, with similar gradients found. Differences are found with the younger 2 Gyr old SSP models, with sMILES models predicting a larger change in both indices with increasing  $[\alpha/\text{Fe}]$ , particularly for the highest metallicities. These differences originate from both larger Mg<sub>b</sub> line strength changes and smaller Fe5270 and Fe5335 line strength changes for an increase of  $[\alpha/\text{Fe}]$  in sMILES models, compared to V+15 models (see Table 3 of Knowles et al. 2023).

However, as we note in Knowles et al. (2023), sMILES and V+15 SSP models deviate the most in young, high metallicity and high  $[\alpha/\text{Fe}]$  stellar populations.

We investigate these trends further, for the wider range of  $[\alpha/\text{Fe}]$  values available for sMILES SSPs, in Figure 11 of Knowles et al. (2023), where we uncover non-monotonic behaviour.

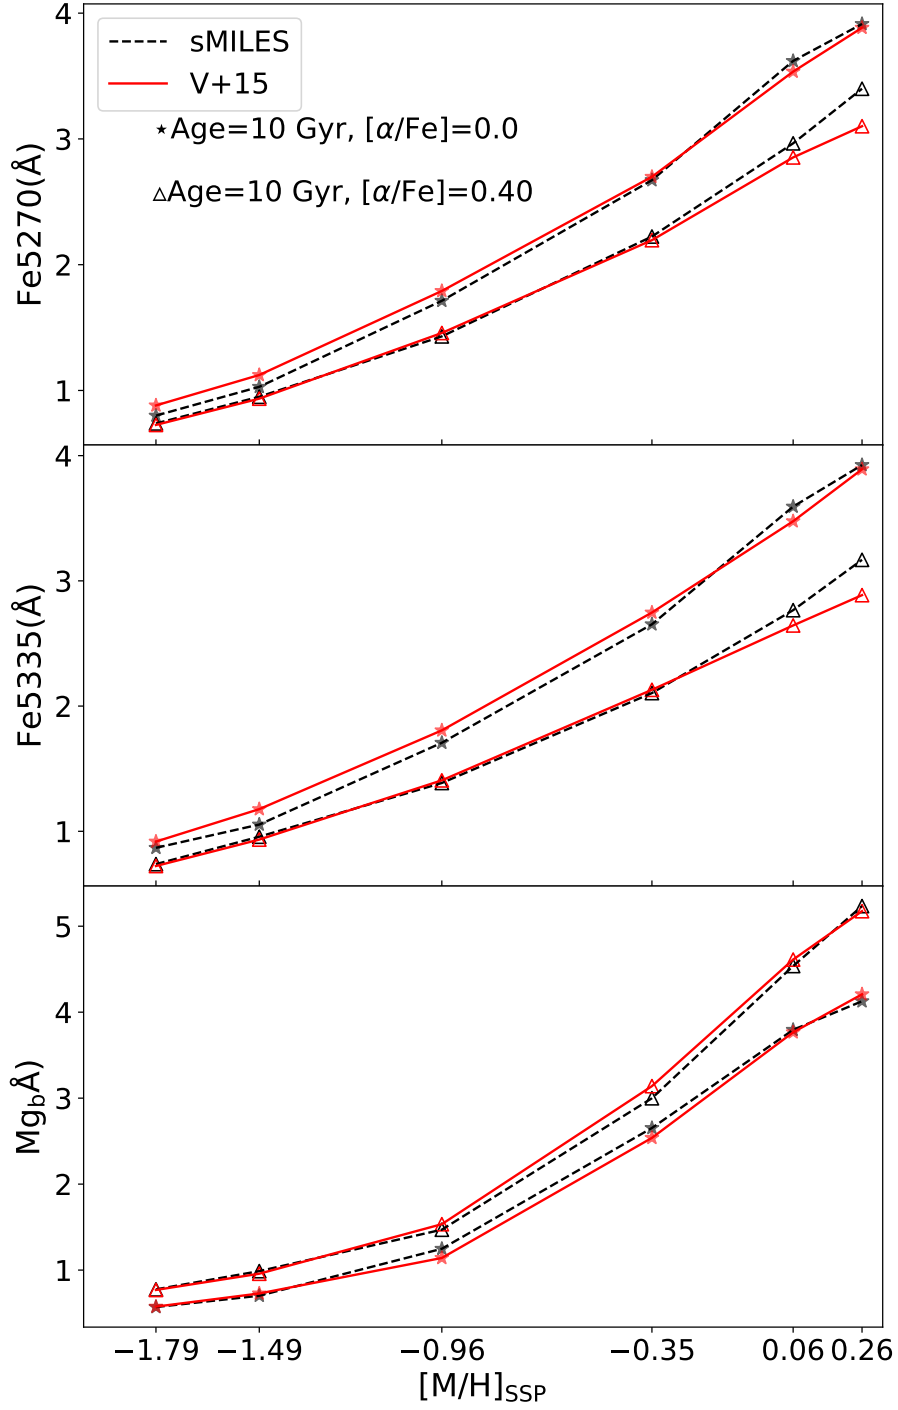

Figure S4: sMILES and V+15 SSP predictions of Fe5270 (Top panel), Fe5333 (Middle panel) and  $\text{Mg}_b$  (Bottom panel) index variations with changing  $[M/H]_{\text{SSP}}$ . The SSPs are 10 Gyr old, with a Universal Kroupa IMF. Index values are measured at MILES FWHM ( $2.5\text{\AA}$ ) resolution.

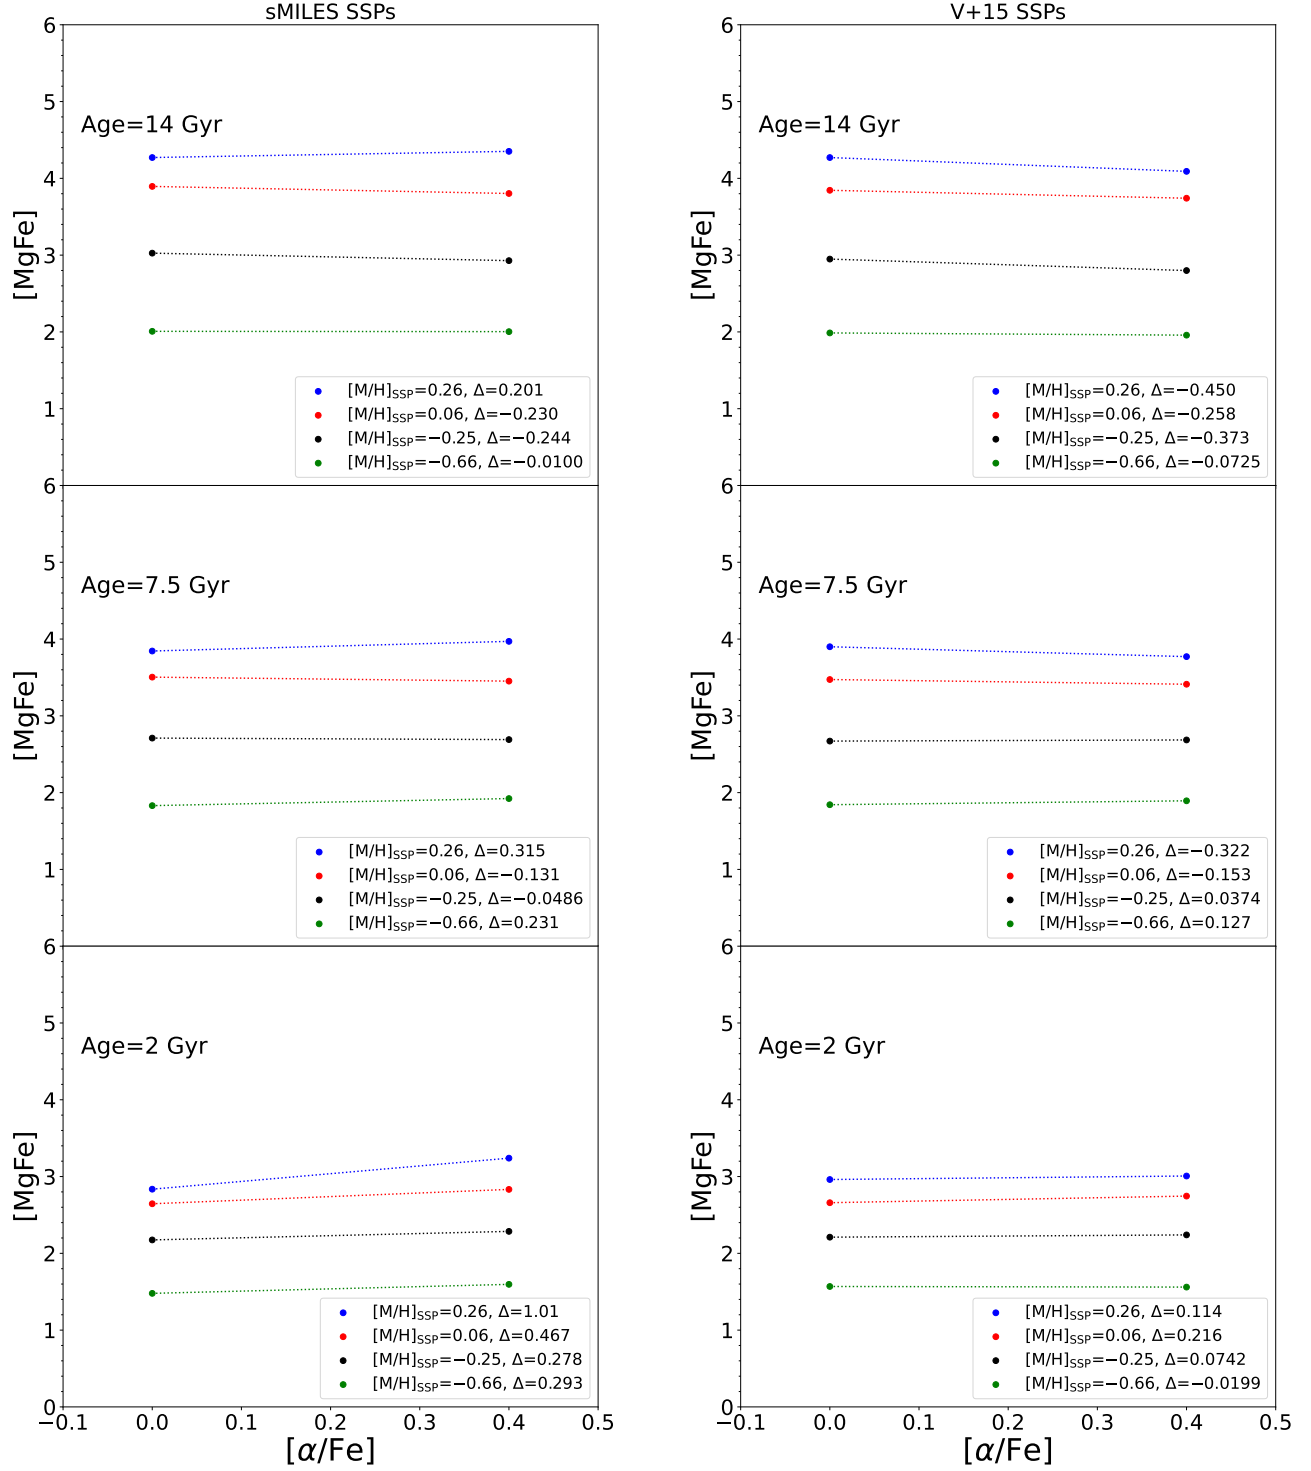

Figure S5: Difference in  $[\text{MgFe}]$  strength between sMILES and V+15 SSP models for 3 ages and 4 metallicities at  $[\alpha/\text{Fe}]=0.0$  and  $0.4$ . Left and right panels show the  $[\text{MgFe}]$  values of sMILES and V+15 SSP models, respectively. The gradient of the line between  $[\text{MgFe}]$  values of  $[\alpha/\text{Fe}]=0.0$  and  $0.4$  models is given, in units of  $\text{\AA} \text{ dex}^{-1}$ . Index values are measured at MILES FWHM ( $2.5\text{\AA}$ ) resolution.

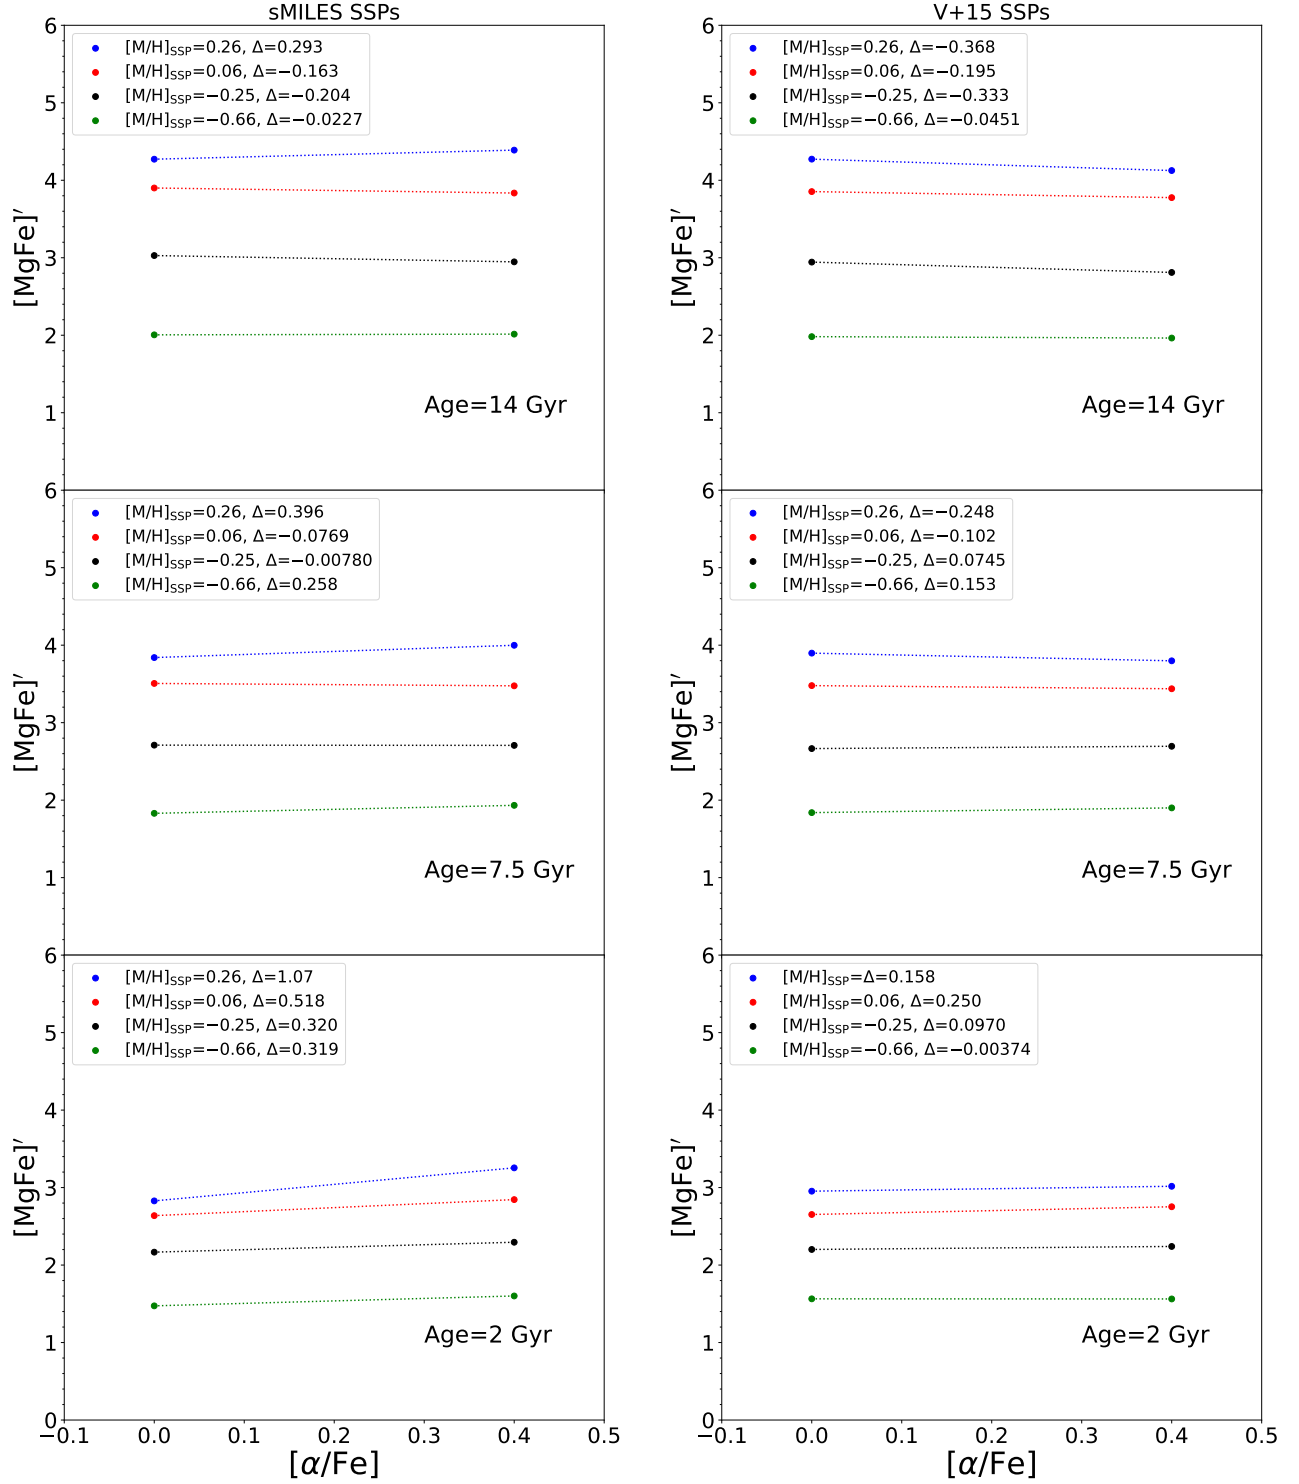



## References

- Cervantes, J. L. and Vazdekis, A. (2009), ‘An optimized  $H\beta$  index for disentangling stellar population ages’, *MNRAS* **392**, 691–704.
- Coelho, P., Barbuy, B., Meléndez, J., Schiavon, R. P. and Castilho, B. V. (2005), ‘A library of high resolution synthetic stellar spectra from 300 nm to 1.8  $\mu\text{m}$  with solar and  $\alpha$ -enhanced composition’, *A&A* **443**, 735–746.
- Coelho, P., Bruzual, G., Charlot, S., Weiss, A., Barbuy, B. and Ferguson, J. W. (2007), ‘Spectral models for solar-scaled and  $\alpha$ -enhanced stellar populations’, *MNRAS* **382**, 498–514.
- González, J. J. (1993), Line strength gradients and kinematic profiles in elliptical galaxies, PhD thesis, Thesis (PH.D.)–UNIVERSITY OF CALIFORNIA, SANTA CRUZ, 1993. Source: Dissertation Abstracts International, Volume: 54-05, Section: B, page: 2551.
- Knowles, A. T., Sansom, A. E., Allende Prieto, C. and Vazdekis, A. (2021), ‘sMILES: a library of semi-empirical MILES stellar spectra with variable  $[\alpha/\text{Fe}]$  abundances’, *MNRAS* **504**(2), 2286–2311.
- Thomas, D., Maraston, C. and Bender, R. (2003), ‘Stellar population models of Lick indices with variable element abundance ratios’, *MNRAS* **339**, 897–911.
- Vazdekis, A., Coelho, P., Cassisi, S., Ricciardelli, E., Falcón-Barroso, J., Sánchez-Blázquez, P., La Barbera, F., Beasley, M. A. and Pietrinferni, A. (2015), ‘Evolutionary stellar population synthesis with MILES - II. Scaled-solar and  $\alpha$ -enhanced models’, *MNRAS* **449**, 1177–1214.
- Worthey, G. (1994), ‘Comprehensive stellar population models and the disentanglement of age and metallicity effects’, *ApJS* **95**, 107–149.
